# Supplementary material for: Orientation-dependent propulsion of active Brownian spheres: from self-advection to programmable cluster shapes
Source: arXiv:2210.13357 ancillary file (2022-10-24)
Supplement: Supplementary file 1 [file SM.pdf]

# Orientation-dependent propulsion of active Brownian spheres: from self-advection to programmable cluster shapes

## Supplemental Material

Stephan Bröker,[1,*] Jens Bickmann,[1,*] Michael te Vrugt,[1] Michael E. Cates,[2] and Raphael Wittkowski[1,†]

[1] *Institut für Theoretische Physik, Center for Soft Nanoscience, Westfälische Wilhelms-Universität Münster, 48149 Münster, Germany*

[2] *DAMTP, Centre for Mathematical Sciences, University of Cambridge, Cambridge CB3 0WA, United Kingdom*

## I. DERIVATION OF ANALYTICAL MODEL

Here, we present in more detail the microscopic derivation of the field-theoretical model given by Eq. (3) from the main text. For this derivation, we make use of the interaction-expansion method [1–6]. Apart from the fact that the propulsion speed $v_\mathrm{A}$ depends on the angle $\phi$ in this work, the derivation is similar to the one presented in Ref. [3]. This allows us to re-use many interim steps and results from Ref. [3], which will therefore not be reproduced here.

Our starting point is the Smoluchowski equation corresponding to the Langevin equations (1) and (2) of the main text, which is given by

$$\dot{\mathfrak{P}} = \sum_{i=1}^{N} \big(D_\mathrm{T}\boldsymbol{\nabla}^2_{\boldsymbol{r}_i} + D_\mathrm{R}\partial^2_{\phi_i}\big)\mathfrak{P} - \boldsymbol{\nabla}_{\boldsymbol{r}_i}\cdot\big(v_\mathrm{A}(\phi_i)\hat{\boldsymbol{u}}(\phi_i)\mathfrak{P} + \boldsymbol{v}_{\mathrm{int},i}(\{\boldsymbol{r}_i\})\mathfrak{P}\big), \tag{1}$$

where $\mathfrak{P}(\{\boldsymbol{r}_i\},\{\phi_i\},t)$ is the many-particle probability density and $\partial_{\phi_i}$ the partial derivative with respect to $\phi_i$. Equation (1) is integrated over the degrees of freedom of all particles except for one. This gives

$$\dot{\varrho}(\boldsymbol{r},\hat{\boldsymbol{u}},t) = \big(D_\mathrm{T}\boldsymbol{\nabla}^2_{\boldsymbol{r}} + D_\mathrm{R}\partial^2_{\phi} - v_\mathrm{A}(\phi)\hat{\boldsymbol{u}}(\phi)\cdot\boldsymbol{\nabla}_{\boldsymbol{r}}\big)\varrho(\boldsymbol{r},\hat{\boldsymbol{u}},t) + \mathcal{I}_\mathrm{int}(\boldsymbol{r},\hat{\boldsymbol{u}},t) \tag{2}$$

with the position-, orientation-, and time-dependent particle number density

$$\varrho(\boldsymbol{r},\hat{\boldsymbol{u}},t) = N\bigg(\prod_{\substack{j=1\\ j\neq i}}^{N}\int_{\mathbb{R}^2}\!\mathrm{d}^2r_j\int_0^{2\pi}\!\mathrm{d}\phi_j\bigg)\mathfrak{P}\bigg|_{\substack{\boldsymbol{r}_i=\boldsymbol{r}\\ \phi_i=\phi}} \tag{3}$$

and the interaction term [3]

$$\mathcal{I}_\mathrm{int} = \beta D_T\boldsymbol{\nabla}_{\boldsymbol{r}}\cdot\bigg(\varrho(\boldsymbol{r},\phi,t)\int_{\mathbb{R}^2}\!\mathrm{d}^2r'\,U_2'(\lVert\boldsymbol{r}-\boldsymbol{r}'\rVert)\frac{\boldsymbol{r}-\boldsymbol{r}'}{\lVert\boldsymbol{r}-\boldsymbol{r}'\rVert}\int_0^{2\pi}\!\mathrm{d}\phi'\,g(\boldsymbol{r},\boldsymbol{r}',\phi,\phi',t)\varrho(\boldsymbol{r}',\phi',t)\bigg), \tag{4}$$

where $U_2'(r)\equiv\mathrm{d}U_2(r)/\mathrm{d}r$ with $r=\lVert\boldsymbol{r}-\boldsymbol{r}'\rVert$.

The interaction term depends on the pair-distribution function

$$g(\boldsymbol{r},\boldsymbol{r}',\phi,\phi',t) = \frac{\varrho^{(2)}(\boldsymbol{r},\boldsymbol{r}',\phi,\phi',t)}{\varrho(\boldsymbol{r},\phi,t)\varrho(\boldsymbol{r}',\phi',t)}, \tag{5}$$

where $\varrho^{(2)}(\boldsymbol{r},\boldsymbol{r}',\phi,\phi',t)$ is the two-particle density. To close Eq. (2), one requires an expression for $g$. We here use the one obtained in Ref. [7], which is translationally, rotationally, and temporally invariant.

Next, a Cartesian orientational expansion [8, 9] of $\varrho(\boldsymbol{r},\hat{\boldsymbol{u}},t)$ with respect to $\hat{\boldsymbol{u}}$ is performed and truncated at second order. This gives

$$\varrho(\boldsymbol{r},\phi,t) \approx \frac{1}{2\pi}\rho(\boldsymbol{r},t) + \frac{1}{\pi}\hat{\boldsymbol{u}}(\phi)\cdot\boldsymbol{P}(\boldsymbol{r},t) + \mathcal{O}(\hat{\boldsymbol{u}}^2) \tag{6}$$

---

* These two authors contributed equally.

† Corresponding author: raphael.wittkowski@uni-muenster.de

with the concentration field

$$\rho(\boldsymbol{r},t) = \int_0^{2\pi}\mathrm{d}\phi\, \varrho(\boldsymbol{r},\phi,t) \tag{7}$$

and the local polarization

$$\boldsymbol{P}(\boldsymbol{r},t) = \int_0^{2\pi}\mathrm{d}\phi\, \hat{\boldsymbol{u}}(\phi)\varrho(\boldsymbol{r},\phi,t). \tag{8}$$

Now, we come to the main difference to the derivation from Ref. [3]: Since we allow also $v_{\mathrm{A}}$ to depend on $\phi$, we perform the Cartesian orientational expansion also for $v_{\mathrm{A}}$. This gives

$$v_{\mathrm{A}}(\phi)\hat{\boldsymbol{u}}(\phi) = \boldsymbol{\mu}^{(1)} + \hat{\boldsymbol{u}}(\phi)\cdot \underline{\mu}^{(2)} + \mathcal{O}(\hat{\boldsymbol{u}}^2) \tag{9}$$

with the orientation-averaged propulsion velocity

$$\boldsymbol{\mu}^{(1)} = \frac{1}{2\pi}\int_0^{2\pi}\mathrm{d}\phi\; v_{\mathrm{A}}(\phi)\hat{\boldsymbol{u}}(\phi) \tag{10}$$

and the symmetric velocity tensor

$$\underline{\mu}^{(2)} = \frac{1}{\pi}\int_0^{2\pi}\mathrm{d}\phi\, v_{\mathrm{A}}(\phi)\hat{\boldsymbol{u}}(\phi)\otimes\hat{\boldsymbol{u}}(\phi). \tag{11}$$

Inserting Eqs. (6) and (9) into Eq. (2) gives two coupled equations for the time evolution of $\rho$ and $\boldsymbol{P}$. These equations involve convolution integrals resulting from the interaction term (4). We can remove these convolution integrals using a combined Fourier and gradient expansion [10].

To obtain, from the resulting two equations, a model that depends only on one order parameter $\rho$, we use a quasi-stationary approximation (QSA) [1, 3, 11]. The idea of the QSA is that conserved quantities relax much slower than nonconserved quantities, such that the latter can be seen as fully relaxed on a sufficiently large time scale. In our case, the concentration field $\rho$ is a conserved quantity, whereas the polarization $\boldsymbol{P}$ is not. Neglecting terms of third or higher order in spatial derivatives, the QSA finally leads to the advection-diffusion model given by Eqs. (3) and (4) in the main text. In this model, the coefficients $c_i$ are given by

$$c_1 = \frac{A(1,0,0)}{\pi}, \tag{12}$$

$$c_2 = \frac{4A(0,1,0)(A(0,1,0)+A(0,1,-1))}{\pi^2 D_{\mathrm{R}}}, \tag{13}$$

$$c_3 = -\frac{3A(0,1,0)+A(0,1,-1)}{\pi D_{\mathrm{R}}}. \tag{14}$$

They contain the interaction coefficients $A(n,k_1,k_2)$ that stem from the interaction-expansion method and are defined as [3]

$$A(n,k_1,k_2) = \frac{-\beta D_{\mathrm{T}}}{(1+\delta_{k_1,0})(1+\delta_{k_2,0})}\int_0^{\infty}\mathrm{d}r\, r^{n+1}U_2'(r)\int_0^{2\pi}\mathrm{d}\theta_1\int_0^{2\pi}\mathrm{d}\theta_2\, g(r,\theta_1,\theta_2)\cos(k_1\theta_1+k_2\theta_2), \tag{15}$$

where $\delta_{ij}$ denotes the Kronecker delta.

## II. COMPUTER SIMULATIONS

All figure numbers refer to the main text.

### A. General

For the Brownian dynamics simulations, we numerically integrated the overdamped Langevin equations (Eqs. (1) and (2) in the main text) using a modified version of the molecular dynamics code LAMMPS [12]. We measure lengths,

times, and energies in terms of the particle diameter $a$, the Lennard-Jones time scale $\tau_{\mathrm{LJ}} = a^2/(\varepsilon\beta D_{\mathrm{T}})$, and the interaction strength $\varepsilon$, respectively.

If not stated otherwise, a quadratic simulation domain with periodic boundary conditions and an edge length of $256a$ was used. Starting from a homogeneous, random initial distribution of the particles, an initial period of $500\tau_{\mathrm{LJ}}$ was simulated. After this initial relaxation, the data were extracted over the following period of $1000\tau_{\mathrm{LJ}}$ using a time step size of $5\cdot 10^{-5}\tau_{\mathrm{LJ}}$, which results in $3\cdot 10^{7}$ time steps in total. In the cases where the form of particle clusters was examined, we discarded an initial period of $1000\tau_{\mathrm{LJ}}$ to ensure a full relaxation of the clusters.

### B. Figure 1

To determine the advection velocity $\boldsymbol{v}_{\mathrm{c}}$ of clusters, we set the propulsion speed to $v_{\mathrm{A},n}(\phi) = v_{\mathrm{A},1}(\phi)$ and varied the angular modulation amplitude $\nu$. We carried out six simulations for each value of $\nu$. In each simulation, we extracted the velocity of the center of the cluster averaged over a period of $1000\tau_{\mathrm{LJ}}$. We then averaged these velocities over the six simulations and calculated the standard deviation. The standard deviation was smaller than $\bar{v}/100$ and is thus negligibly small.

### C. Figure 2

The coefficients $c_1$, $c_2$, and $c_3$ required for evaluating the analytical prediction for the spinodal can be obtained from Eqs. (12)–(14). They are defined in terms of the coefficients $A(n,k_1,k_2)$ given by Eq. (15). These, in turn, are defined via the pair-distribution function $g$, for which (since the Weeks-Chandler-Andersen potential is used) we can employ the representation from Ref. [7]. The required coefficients are approximately given by

$$A(1,0,0) = \big(38.2 + 18.4e^{2.87\Phi}\big)\frac{a^4}{\tau_{\mathrm{LJ}}}, \tag{16}$$

$$A(0,1,0) = 36.9\frac{a^3}{\tau_{\mathrm{LJ}}}, \tag{17}$$

$$A(0,1,-1) = \big(-0.232 - 13.6\Phi\big)\frac{a^3}{\tau_{\mathrm{LJ}}}. \tag{18}$$

Each state diagram was calculated by varying the Péclet number Pe and the overall packing density $\Phi_0$ and determining for each of these parameter combinations the reduced average interaction energy per particle $E_{\mathrm{int}}/(\varepsilon N)$. The reduced interaction energy was extracted every $5\tau_{\mathrm{LJ}}$ for every particle and averaged over the particles and over the different points in time. Further details on the interaction potential energy can be found in Ref. [2].

### D. Figure 3

The deformation of clusters for different values of the angular modulation amplitude $\nu$ in the case $n = 2$ with the corresponding propulsion velocity $v_{\mathrm{A},n}(\phi) = v_{\mathrm{A},2}(\phi)$ was calculated using a simulation domain whose form also depends on $\nu$. For strong values of $\nu$, the clusters become elliptic with a high eccentricity. In some cases, they can thus become wider than the simulation domain. For periodic boundaries, this results in a belt of particles rather than an elliptic cluster. To avoid this, we used a rectangular simulation domain whose aspect ratio was chosen as $p = 1+25\nu/3$. The resulting width and height are $256a\sqrt{p}$ and $256a/\sqrt{p}$, respectively. Ten simulations were performed for each value of $\nu$. The height and width of the elliptic clusters were calculated by fitting the function

$$h(x) = \frac{\tanh(u_{\mathrm{st}}(u_{\mathrm{bo}} - x)) + 1}{2}\frac{\tanh(l_{\mathrm{st}}(x - l_{\mathrm{bo}})) + 1}{2}h_{\max} + h_{\min} \tag{19}$$

to the smoothed density distribution $\Phi_{\mathrm{smo}}$. The parameters $h_{\max}$ and $h_{\min}$ denote the maximal and minimal values of $\Phi_{\mathrm{smo}}$, $u_{\mathrm{st}}$ and $l_{\mathrm{st}}$ determine the steepness of the upper and lower flanks of the smoothed density, respectively, and $u_{\mathrm{bo}}$ and $l_{\mathrm{bo}}$ denote the upper and lower positions of the flanks of the density. The function was fitted along the $x$-dimension and the $y$-dimension, and the distance $|u_{\mathrm{bo}} - l_{\mathrm{bo}}|$ between the flanks was taken as the width and height of the clusters, respectively.

The smoothed density distribution $\Phi_{\mathrm{smo}}$ was calculated through a convolution of the particle positions with the smoothing function

$$c(r) = \begin{cases} \bar{c}\exp\big(\frac{-1}{1-(r/r_{\mathrm{c}})^2}\big), & \text{if } r < r_{\mathrm{c}}, \\ 0, & \text{else}, \end{cases} \tag{20}$$

where we chose $r_{\mathrm{c}} = 5a$ as the cut-off distance. The parameter $\bar{c}$ is a normalization parameter used to preserve the average packing density. We extracted the values of the height and width every $10\tau_{\mathrm{LJ}}$ and averaged over all simulations corresponding to the considered value of $\nu$ and over time. For each value of $\nu$, we performed 5 (for $\nu < 1/4$) or 10 (for $\nu \geq 1/4$) simulations. Some simulations had to be discarded (in particular for large $\nu$) as the particles were either not fully relaxed to a single elliptic cluster or a belt has formed despite the use of a wider simulation domain. For every data point, at least 65 different measurements were taken into account.

### E. Figure 4

The density fields shown in the bottom row of Fig. 4 were calculated by performing eleven different simulations for each value of $n$ and $\nu$ and calculating the smoothed density distribution every $50\tau_{\mathrm{LJ}}$. The resulting smoothed density distributions were averaged over all simulations corresponding to the considered value of $\nu$ and over time after the particle positions were shifted to the center, such that the clusters would overlap. Up to four of the eleven simulations had to be discarded because the system did not fully relax within the simulation time. The simulation domain used for $n = 2$ had a width of $384a$ and a height of $128a$, whereas the simulation domain used for $n = 3, 4$ was quadratic with an edge length of $384a$.

### F. Figure 5

The local polarization $\boldsymbol{P}(\boldsymbol{r})$ and local density current $\boldsymbol{J}(\boldsymbol{r})$ are defined as

$$\boldsymbol{P}(\boldsymbol{r}) = \sum_{i=0}^{N_{\mathrm{part}}} \hat{\boldsymbol{u}}_i c(\|\boldsymbol{r} - \boldsymbol{r}_i\|) \tag{21}$$

and

$$\boldsymbol{J}(\boldsymbol{r}) = \sum_{i=0}^{N_{\mathrm{part}}} \boldsymbol{v}_i c(\|\boldsymbol{r} - \boldsymbol{r}_i\|) \tag{22}$$

with the position $\boldsymbol{r}_i$, the orientation $\hat{\boldsymbol{u}}_i$, and the velocity $\boldsymbol{v}_i$ of the $i$-th particle. After calculating $\boldsymbol{P}$ and $\boldsymbol{J}$ using Eqs. (21) and (22), we additionally averaged over an area of size $(128a/20) \times (384a/20)$, such that the arrows shown in Fig. 5 represent the local averages of $\boldsymbol{P}$ and $\boldsymbol{J}$. We here use $r_{\mathrm{c}} = 1.5a$ as the cut-off distance for $c(r)$. After an initial relaxation time period of $1000\tau_{\mathrm{LJ}}$, we extracted the smoothed density distribution $\Phi_{\mathrm{smo}}$, the local polarization $\boldsymbol{P}$, and the local density current $\boldsymbol{J}$ every $\tau_{\mathrm{LJ}}$ over a time of $1000\tau_{\mathrm{LJ}}$ for six different simulations resulting in 6000 data points. Similar to Fig. 4, the particle positions and measured data were shifted such that the clusters overlap. Then, we averaged over these 6000 data points. The plot program used for the streamlines (matplotlib pyplot streamplot) requires an equidistant grid. Since the simulations were performed on a rectangular (non-quadratic) domain with 20 data points for each spatial direction, the equidistant grid was created by interpolating along the $x$-direction.

---

[1] R. Wittkowski, J. Stenhammar, and M. E. Cates, Nonequilibrium dynamics of mixtures of active and passive colloidal particles, New Journal of Physics **19**, 105003 (2017).
[2] J. Bickmann, S. Bröker, J. Jeggle, and R. Wittkowski, Analytical approach to chiral active systems: suppressed phase separation of interacting Brownian circle swimmers, Journal of Chemical Physics **156**, 194904 (2022).
[3] J. Bickmann and R. Wittkowski, Predictive local field theory for interacting active Brownian spheres in two spatial dimensions, Journal of Physics: Condensed Matter **32**, 214001 (2020).
[4] J. Bickmann and R. Wittkowski, Collective dynamics of active Brownian particles in three spatial dimensions: a predictive field theory, Physical Review Research **2**, 033241 (2020).

[5] M. te Vrugt, T. Frohoff-Hülsmann, E. Heifetz, U. Thiele, and R. Wittkowski, From a microscopic inertial active matter model to the Schrödinger equation, arXiv:2204.03018 (2022).

[6] M. te Vrugt, J. Bickmann, and R. Wittkowski, How to derive an active field theory: a step-by-step tutorial, in preparation (2022).

[7] J. Jeggle, J. Stenhammar, and R. Wittkowski, Pair-distribution function of active Brownian spheres in two spatial dimensions: simulation results and analytic representation, Journal of Chemical Physics **152**, 194903 (2020).

[8] M. te Vrugt and R. Wittkowski, Relations between angular and Cartesian orientational expansions, AIP Advances **10**, 035106 (2020).

[9] M. te Vrugt and R. Wittkowski, Orientational order parameters for arbitrary quantum systems, Annalen der Physik **532**, 2000266 (2020).

[10] A. J. M. Yang, P. D. Fleming, and J. H. Gibbs, Molecular theory of surface tension, Journal of Chemical Physics **64**, 3732 (1976).

[11] M. E. Cates and J. Tailleur, When are active Brownian particles and run-and-tumble particles equivalent? Consequences for motility-induced phase separation, EPL **101**, 20010 (2013).

[12] S. Plimpton, Fast parallel algorithms for short-range molecular dynamics, Journal of Computational Physics **117**, 1 (1995).
